# Supplementary material for: OOOE: Only-One-Object-Exists Assumption to Find Very Small Objects in Chest Radiographs
Source: arXiv:2210.06806 source file (2022-10-13)
Supplement: Supplementary file 4 [file imp_details.tex]

\begin{table}[t]
\centering   

\setlength{\tabcolsep}{3pt}
\small
\caption{Implementation Details}
\label{table:imp_details}
\begin{tabular}{l|l||l|l}
\toprule
\textbf{Optimizer}     & SGD (momentum 0.9) &           \textbf{Backbone} &          \texttt{resnet34} + FPN  \\
\midrule
\textbf{Learning rate} &                                  0.04 &  \textbf{Init weight} &                ImageNet pretrained\\
\midrule
\textbf{Train epoch}   &                                    40 &               \textbf{GPUs} &  NVIDIA RTX 2080 Ti * 8 \\
\midrule
\textbf{LR drop} & $\times$ 0.1 at 30$^{\text{th}}$ epoch  &         \textbf{Batch size} &                     192 \\
\bottomrule
\end{tabular}
\end{table}
